# Supplementary material for: Path Integral Approach Unveils the Role of Complex Energy Landscape for Activated Dynamics of Glassy Systems
Source: arXiv:2012.09556 ancillary file (2021-09-09)
Supplement: Supplementary file 1 [file alternative-init.pdf]

```

(*****
    *****)
(*****initialization close to the  $\beta=$ 
  0 solution *****)
(*****
    *****)

```

(\* In this case it is convenient to fix the  
parameter a of the free solution,  
see manuscript \*)

a = .999999;

$$T = \text{Chop} \left[ \frac{\text{Log} \left[ \frac{\sqrt{-1-\sqrt{a}}}{\sqrt{-1+\sqrt{a}}} \right]}{\sqrt{a}} / 2 \right];$$

(\* Tau associated to a, see manuscript \*)

dt = T / n; (\* corresponding dt \*)

$\beta = 0.5$ ; (\* this should be sufficiently close to  $\beta=$   
0 for the algorithm to converge \*)

dif = Table[i - j, {i, 1, 2 n + 1}, {j, 1, 2 n + 1}];

(\* dif[x,y]=x-y \*)

sum = Table[i + j - 2 (n + 1), {i, 1, 2 n + 1},  
{j, 1, 2 n + 1}]; (\* sum[x,y]=x+y \*)

CC = Cosh[ $a^{1/2}$  dt dif] -  $a^{-1/2}$  Sinh[ $a^{1/2}$  dt Abs[dif]];

(\* exact analytic expressions \*)

CC[[1, 2 n + 1]] = 0.0;

```

(* these will not be updated by the code,
they should be set to zero *)
CC[[2 n + 1, 1]] = 0.0;
(* these will not be updated by the code,
they should be set to zero *)
ThR = CC / 2; (* exact analytic expressions *)
T2hX = CC / 4 + IdentityMatrix[2 n + 1] (-1 / (2 dt));
(* exact analytic expressions *)
Ctot = ArrayFlatten[{{CC, ThR}, {ThR, T2hX}}];
(* Fast funciont to join matrices *)
Ctot = Developer`ToPackedArray[Ctot];
(* convert to a Packed Array for efficiency *)

CCdt = ((1 - a)1/2 Cosh[a1/2 dt dif] + Cosh[a1/2 dt sum])
      (1 - a)1/2 / a;
CCdt[[1, 2 n + 1]] = 0.0;
(* these will not be updated by the code,
they should be set to zero *)
CCdt[[2 n + 1, 1]] = 0.0;
(* these will not be updated by the code,
they should be set to zero *)
ThRdt = CCdt / 2;
T2hXdt = CCdt / 4;
Ctotdt = ArrayFlatten[
  {{CCdt, ThRdt}, {ThRdt, T2hXdt}}];
(* Fast funciont to join matrices *)
Ctotdt = Developer`ToPackedArray[Ctotdt];

βμ = Table[1., {i, 1, 2 nin + 1}];
(* exact analytic expressions *)
βμt = (a - 1) / 2 βμ; (* exact analytic expressions *)

```



```

CC = Take[Ctot, 2 ns + 1, 2 ns + 1];
ThR2 = Take[Ctot, 2 ns + 1, -(2 ns + 1)];
ThR1 = Take[Ctot, -(2 ns + 1), 2 ns + 1];
T2hX = Take[Ctot, -(2 ns + 1), -(2 ns + 1)];
CCdt = Take[Ctotdt, 2 ns + 1, 2 ns + 1];
ThR2dt = Take[Ctotdt, 2 ns + 1, -(2 ns + 1)];
ThR1dt = Take[Ctotdt, -(2 ns + 1), 2 ns + 1];
T2hXdt = Take[Ctotdt, -(2 ns + 1), -(2 ns + 1)];

```

```
(* resampling *)
```

```
(***** taking care of the singularity on the
diagonal *****)
```

```

DD = LowerTriangularize[CC] +
      UpperTriangularize[2 - CC, 1];
nDD = ArrayResample[DD, {2 n + 1, 2 n + 1}];
nCC = LowerTriangularize[nDD] +
      Transpose[LowerTriangularize[nDD, -1]];

```

```

DD = LowerTriangularize[ThR2] +
      UpperTriangularize[1 - ThR2, 1];
nDD = ArrayResample[DD, {2 n + 1, 2 n + 1}];
nThR2 = LowerTriangularize[nDD] +
      Transpose[LowerTriangularize[nDD, -1]];

```

```
(** ThR1 and ThR2 are more complicated because
the diagonal is constant but they are not
symmetric **)
```

```

DD1 = LowerTriangularize[ThR1] +
      UpperTriangularize[1 - ThR2, 1];
nDD1 = ArrayResample[DD1, {2 n + 1, 2 n + 1}];
DD2 = LowerTriangularize[ThR2] +
      UpperTriangularize[1 - ThR1, 1];

```

```

nDD2 = ArrayResample[DD2, {2 n + 1, 2 n + 1}];

nThR1 = LowerTriangularize[nDD1] +
  Transpose[LowerTriangularize[nDD2, -1]];
nThR2 = LowerTriangularize[nDD2] +
  Transpose[LowerTriangularize[nDD1, -1]];

(** T2hX is more complicated because it is
    symmetric but the diagonal is not constant **)
mat = T2hX + IdentityMatrix[2 ns + 1] / (2 dts);
diam = DiagonalMatrix[Diagonal[mat]-1/2];
rmat = diam.mat.diam;
(* I resample a matrix with diagonal equal
   to one *)
DD = LowerTriangularize[rmat] +
  UpperTriangularize[2 - rmat, 1];
nDD = ArrayResample[DD, {2 n + 1, 2 n + 1}];
nrmat = LowerTriangularize[nDD] +
  Transpose[LowerTriangularize[nDD, -1]];
ndiap = DiagonalMatrix[
  ArrayResample[Diagonal[mat]1/2, 2 n + 1]];
nmat = ndiap.nrmat.ndiap;
(* I go back to the original matrix *)
nT2hX = nmat - IdentityMatrix[2 n + 1] / (2 dt);

(* resampled solution *)

nCtot = ArrayFlatten[{{nCC, nThR2}, {nThR1, nT2hX}}];

nCCdt = ArrayResample[CCdt, {2 n + 1, 2 n + 1}];
nThR2dt = ArrayResample[ThR2dt, {2 n + 1, 2 n + 1}];

```

```

nThR1dt = ArrayResample[ThR1dt, {2 n + 1, 2 n + 1}];
nT2hXdt = ArrayResample[T2hXdt, {2 n + 1, 2 n + 1}];
nCtotdt = ArrayFlatten[
  {{nCCdt, nThR2dt}, {nThR1dt, nT2hXdt}}];

nβμ = ArrayResample[βμ, 2 nin + 1];
nβμt = ArrayResample[βμt, 2 nin + 1];

{Ctot, Ctotdt, βμ, βμt} = {nCtot, nCtotdt, nβμ, nβμt};

(* quantities that may have been messed up
   by the resampling are set to the correct
   values *)

(* diagonals *)
Do[Ctot[[i, i]] = 1.0;
  Ctot[[i, 2 n + 1 + i]] = 0.5;
  Ctot[[2 n + 1 + i, i]] = 0.5;; {i, 1, 2 n + 1}];

(* corners will not be updated by the algorithm *)
Ctotdt[[1, 1]] = 1.0;
Ctotdt[[2 n + 1, 2 n + 1]] = 1.0;
Ctotdt[[1, 2 n + 1 + 1]] = 0.5;
Ctotdt[[2 n + 1 + 1, 1]] = 0.5;

Ctotdt[[2 n + 1, 2 (2 n + 1)]] = 0.5;
Ctotdt[[2 (2 n + 1), 2 n + 1]] = 0.5;

Ctot[[2 n + 2, 2 n + 2]] = (1 + β2 3 / 2) / 4 - 1 / (2 dt);
(* β must have been defined *)

```

```

Ctot[[2 (2 n + 1), 2 (2 n + 1)]] =
  (1 +  $\beta^2$  3 / 2) / 4 - 1 / (2 dt);
Ctotdt[[2 n + 2, 2 n + 2]] = (1 +  $\beta^2$  3 / 2) / 4;
Ctotdt[[2 (2 n + 1), 2 (2 n + 1)]] = (1 +  $\beta^2$  3 / 2) / 4;

```

```
(* symmetrization *)
```

```

FullSym[Ctot];
FullSym[Ctotdt];
SymV[ $\beta\mu$ ];
SymV[ $\beta\mu t$ ];

```

```
(* {Ctot,Ctotdt, $\beta\mu$ , $\beta\mu t$ } is ready to be feed
to the Newton-Krylov algorithm *)
```
