# Supplementary material for: Path Integral Approach Unveils the Role of Complex Energy Landscape for Activated Dynamics of Glassy Systems
Source: arXiv:2012.09556 ancillary file (2021-09-09)

```
(* this code compute the solution through the  
  Newton-Krylov algorithm initialized with  
  an approximate solution,  
use freely citing the original paper *)
```

In[•]:=

```
(* requires the functions defined in  
  "functions.nb"*)
```

```
SetDirectory[NotebookDirectory[]];  
NotebookEvaluate[  
  FileNameJoin[{Directory[], "functions.nb"}]]];
```

```
n = 100; (* Nt of the manuscript,  
Nt=2000 requires more than 200 giga *)  
nin = n - 1; (* internal indexes,  
see "functions.nb" *)
```

```
dt = 4. / 100; (* the new dt,  
in this case it corresponds to a Tau=4. *)  
 $\beta$  = 1.65; (* the new inverse temperature *)
```

```

(***** matrices
  initialization *****)

(* the matrices are initialized through
  the solution at different values of  $\beta$  and dt,
  in this case the same dt and a different  $\beta=$ 
  1.695 *)

(*****)
{Ctot, Ctotdt,  $\beta\mu$ ,  $\beta\mu t$ } =
  BinaryDeserialize[<< "C1695.100.40"];

(* alternative initialization matrices are
  given in the file "alternative-init.nb"*)

```

```

In[•]:= (* symmetrize the input,
  in principle it should not be necessary
  because it should be already symmetrized *)

FullSym[Ctot];
FullSym[Ctotdt];
SymV[ $\beta\mu$ ];
SymV[ $\beta\mu t$ ];

```

```

In[•]:=

CalcoloEquazioni[];

```

```

(* symmetrizing the output *)
FullSym[equa];
FullSym[equadt];
SymV[equa $\mu$ ];
SymV[equa $\mu$ t];

absq = 1;
While[absq > .0001,
  (* this fixes the precision required *)

  (*****running GMRES *****)
  GMREScomp[.00, 400];
  (* Krylov of size 400 is ok for n=
    2000 and Tau=40,
    for smaller Tau both n and the size can
    be decreased
  *)

  qsol = Sum[yn[[i]] $\times$ q[i], {i, 1, nK - 1}];
  (* approximate solution of the inversion
    of the Jacobian according to GMRES *)

  Clear[q];
  (* clear the Arnoldi base *)

  {dCtot, dCtotdt, d $\beta\mu$ , d $\beta\mu$ t} = IFullComp[qsol];
  (* decompression *)

  (***** Newton
    Update *****)
  {Ctot, Ctotdt,  $\beta\mu$ ,  $\beta\mu$ t} =
    {Ctot, Ctotdt,  $\beta\mu$ ,  $\beta\mu$ t} +

```

```

    {dCtot, dCtotdt, d $\beta\mu$ , d $\beta\mu t$ };

    absq = Max[Abs[qsol]];

    (** Equations **)
    CalcoloEquazioni[];
    FullSym[equa];
    FullSym[equadt];
    SymV[equa $\mu$ ];
    SymV[equa $\mu t$ ];

    Print[absq];
  ];

  (*

  (* Print the output on files *)

  CalcoloEE[]>>"ene165.100.40";
  BinarySerialize[{Ctot,Ctotdt, $\beta\mu$ , $\beta\mu t$ }]>>
    "C165.100.40";

  *)

```

0.237685

0.0193403

0.000052475

```
In[ ]:= ListPlot[ $\beta\mu$ ]  
ListPlot[ $\beta\mu t$ ]  
MatrixPlot[Ctot]  
MatrixPlot[Ctotdt]
```

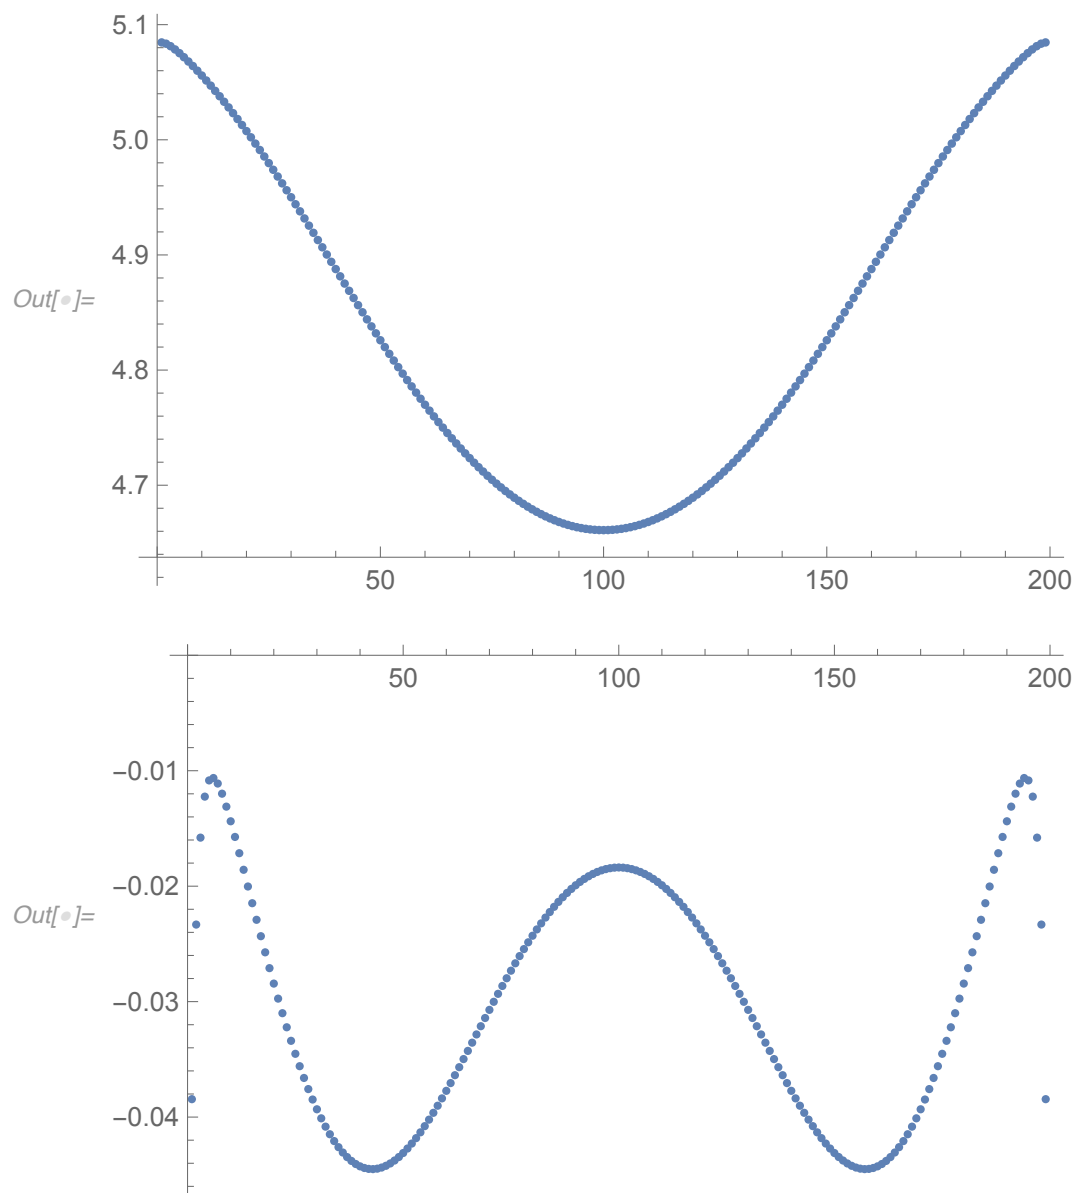

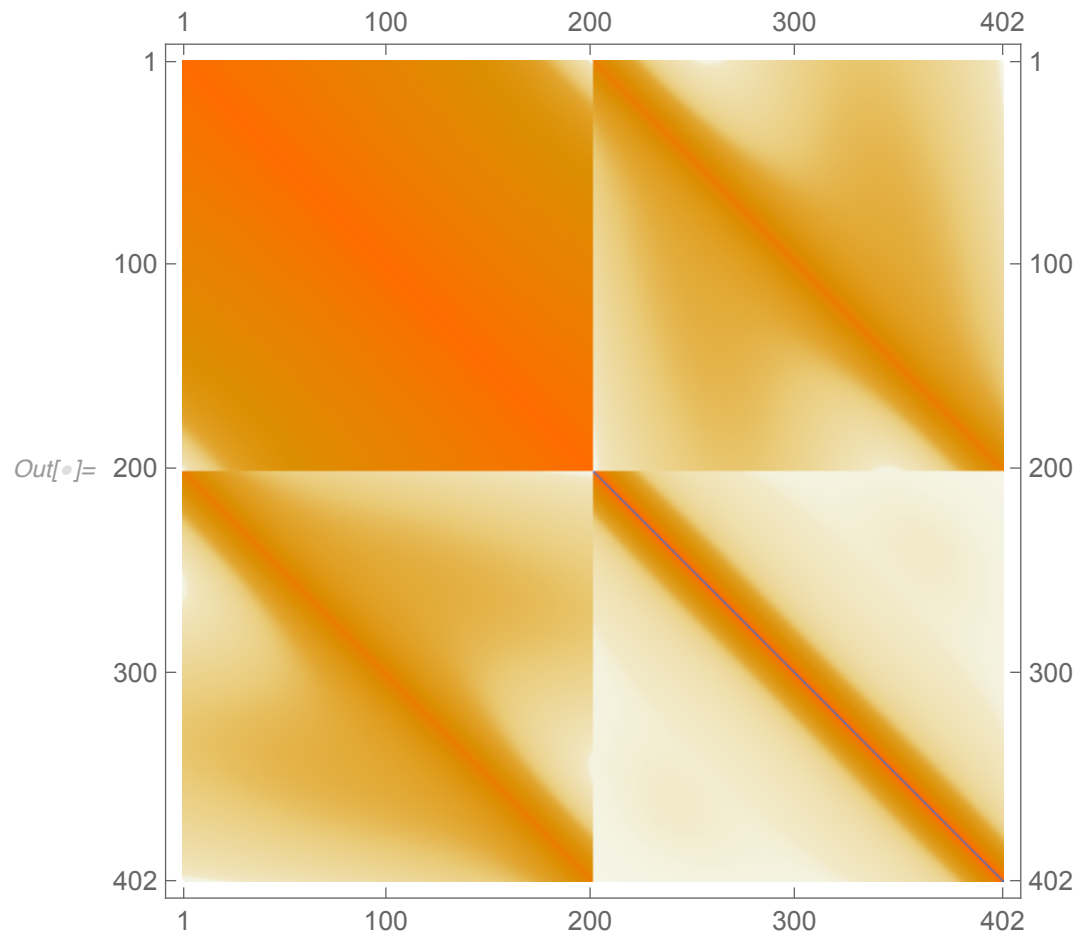

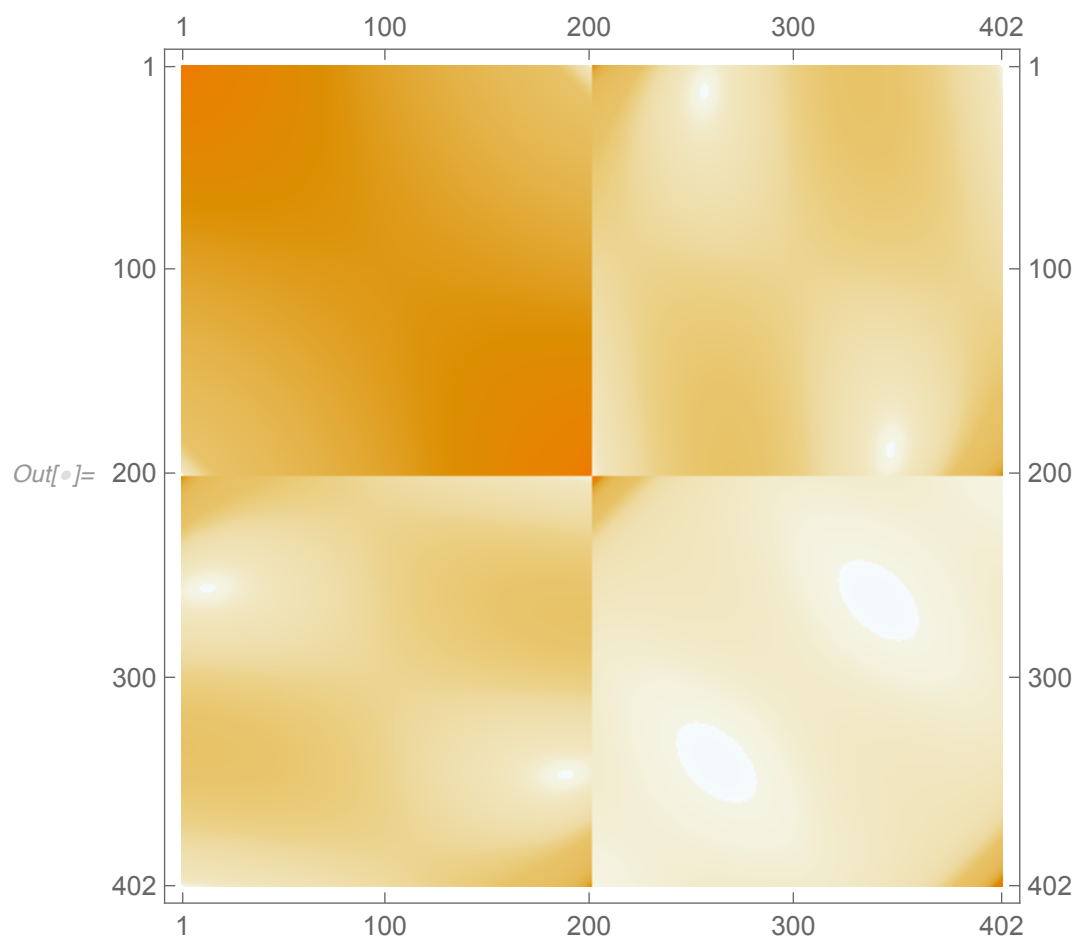

Supplement: Supplementary file 2 [file code.pdf]
