# Supplementary material for: Path Integral Approach Unveils the Role of Complex Energy Landscape for Activated Dynamics of Glassy Systems
Source: arXiv:2012.09556 ancillary file (2021-09-09)
Supplement: Supplementary file 3 [file functions.pdf]

```
(** Functions **)
```

```
CalcoloEquazioni[] := {
```

```
  (* this functions compute the equations *)
```

```
  (*****first it fixes the  
    values of the matrix X on the corners  
    because it will not be changed by the  
    iteration *****)
```

```
Ctot[[2 n + 2, 2 n + 2]] =  $(1 + \beta^2 3 / 2) / 4 - 1 / (2 dt)$ ;
```

```
Ctot[[2 (2 n + 1), 2 (2 n + 1)]] =
```

```
   $(1 + \beta^2 3 / 2) / 4 - 1 / (2 dt)$ ;
```

```
Ctotdt[[2 n + 2, 2 n + 2]] =  $(1 + \beta^2 3 / 2) / 4$ ;
```

```
Ctotdt[[2 (2 n + 1), 2 (2 n + 1)]] =  $(1 + \beta^2 3 / 2) / 4$ ;
```

```
  (***** Computation of the  $\Delta$   
    functions *****)
```

```
CC = Take[Ctot, 2 n + 1, 2 n + 1];
```

```
ThR2 = Take[Ctot, 2 n + 1, -(2 n + 1)];
```

```
ThR1 = Take[Ctot, -(2 n + 1), 2 n + 1];
```

```
T2hX = Take[Ctot, -(2 n + 1), -(2 n + 1)];
```

```
CCdt = Take[Ctotdt, 2 n + 1, 2 n + 1];
```

```
ThR2dt = Take[Ctotdt, 2 n + 1, -(2 n + 1)];
```

```
ThR1dt = Take[Ctotdt, -(2 n + 1), 2 n + 1];
```

```

T2hXdt = Take[Ctotdt, -(2 n + 1), -(2 n + 1)];

(* these formulas are specific for the p=
3 case *)

rCC = 1 / 2 CC2;
ThrR1 = CC Thr1;
ThrR2 = CC Thr2;
T2hrX = CC T2hX + Thr1 Thr2;

(* the matrix is formed in such a way
that the subsequent product is an
ordinary matrix product*)

rCtot =
-3  $\beta^2$  ArrayFlatten[
  {{T2hrX, ThrR1}, {ThrR2, rCC}}];
(*
Developer`PackedArrayQ[rCtot];
(* this test that the output is a
Mathematica PackedArray,
it is essential for efficiency *)
*)

rCCdt = 1 / 2 CCdt2;
ThrR1dt = CCdt Thr1dt;
ThrR2dt = CCdt Thr2dt;
T2hrXdt = CCdt T2hXdt + Thr1dt Thr2dt;

rCtotdt =
-3  $\beta^2$  ArrayFlatten[
  {{T2hrXdt, ThrR1dt}, {ThrR2dt, rCCdt}}];
(*

```

```

Developer`PackedArrayQ[ $\Gamma$ Ctotdt];
*)
(*****)

(*****)
(* Computation of the interaction term *)

(* the formulas are valid for number of
replicas n=0, see manuscript
IMPORTANT: the integrals are written
as a matrix product this means that
we are not satisfying the trapezoidal
rule becose the first and last point
have weight one and not 1/2 as
required. However for n=
0 those terms cancel due to the fact
that the Ctot and Ctotdt are the same
on the border,
for n different from zero one has to
take into account this effect to have
an algorithm with a  $O(\Delta t^2)$  error *)

prod =  $\Gamma$ Ctot.Ctot -  $\Gamma$ Ctotdt.Ctotdt;
proddt =  $\Gamma$ Ctot.Ctotdt +  $\Gamma$ Ctotdt.Ctot -
2  $\Gamma$ Ctotdt.Ctotdt;
prod *= dt;
proddt *= dt;

(* terms depending on the initial and
final condition *)

PP =
Flatten[Take[ $\Gamma$ Ctot, 2 (2 n + 1), {(2 n + 1) + 1}]]  $\times$ 

```

```

    ConstantArray[Take[Ctot, 1][[1]],
      2 (2 n + 1)];
PP +=
  Flatten[Take[TCtot, 2 (2 n + 1), {2 (2 n + 1)}]] ×
    ConstantArray[Take[Ctot, {2 n + 1}][[1]],
      2 (2 n + 1)];

prod += PP;
proddt += PP;

(*
Developer`PackedArrayQ[prod];
Developer`PackedArrayQ[proddt];
(* tests on the interaction term *)
*)

(*****
(* we extract that internal part of the
  interaction terms,
forming two new matrices of size nin *)
prodint = ArrayFlatten[
  {{prod[[2 ;; 2 n, 2 ;; 2 n]],
    prod[[2 ;; 2 n, 2 n + 3 ;; 4 n + 1]]},
  {prod[[2 n + 3 ;; 4 n + 1, 2 ;; 2 n]],
    prod[[2 n + 3 ;; 4 n + 1, 2 n + 3 ;; 4 n + 1]]}}];
prodintdt = ArrayFlatten[
  {{proddt[[2 ;; 2 n, 2 ;; 2 n]],
    proddt[[2 ;; 2 n, 2 n + 3 ;; 4 n + 1]]},
  {proddt[[2 n + 3 ;; 4 n + 1, 2 ;; 2 n]],
    proddt[[2 n + 3 ;; 4 n + 1,
      2 n + 3 ;; 4 n + 1]]}}];
(*****
(* we extract the column vectors of the
  interaction terms,

```

```

the names are self-explanatory *)
pCR1in = Join[prod[[2 ;; 2 n, 1]],
  prod[[2 n + 3 ;; 4 n + 1, 1]]];
pCR1fin = Join[prod[[2 ;; 2 n, 2 n + 1]],
  prod[[2 n + 3 ;; 4 n + 1, 2 n + 1]]];
pR2Xin = Join[prod[[2 ;; 2 n, 2 n + 2]],
  prod[[2 n + 3 ;; 4 n + 1, 2 n + 2]]];
pR2Xfin = Join[prod[[2 ;; 2 n, 4 n + 2]],
  prod[[2 n + 3 ;; 4 n + 1, 4 n + 2]]];

(* we extract the internal part of the
matrices *)
Ctotint = ArrayFlatten[
  {{Ctot[[2 ;; 2 n, 2 ;; 2 n]],
    Ctot[[2 ;; 2 n, 2 n + 3 ;; 4 n + 1]]},
  {Ctot[[2 n + 3 ;; 4 n + 1, 2 ;; 2 n]],
    Ctot[[2 n + 3 ;; 4 n + 1, 2 n + 3 ;; 4 n + 1]]}}];
Ctotintdt = ArrayFlatten[
  {{Ctotdt[[2 ;; 2 n, 2 ;; 2 n]],
    Ctotdt[[2 ;; 2 n, 2 n + 3 ;; 4 n + 1]]},
  {Ctotdt[[2 n + 3 ;; 4 n + 1, 2 ;; 2 n]],
    Ctotdt[[2 n + 3 ;; 4 n + 1,
      2 n + 3 ;; 4 n + 1]]}}];
(*****
(* we extract the column vectors of the
matrices, the names are self-explanatory *)
CR1in = Join[Ctot[[2 ;; 2 n, 1]],
  Ctot[[2 n + 3 ;; 4 n + 1, 1]]];
CR1fin = Join[Ctot[[2 ;; 2 n, 2 n + 1]],
  Ctot[[2 n + 3 ;; 4 n + 1, 2 n + 1]]];
R2Xin = Join[Ctot[[2 ;; 2 n, 2 n + 2]],
  Ctot[[2 n + 3 ;; 4 n + 1, 2 n + 2]]];
R2Xfin = Join[Ctot[[2 ;; 2 n, 4 n + 2]],

```

```

Ctot[[2 n + 3 ;; 4 n + 1, 4 n + 2]]];

(* The matrix containint the second
derivatives is written as an operator
on the interal matrices *)

D2 = SparseArray[
  {{i_, i_} → -2., {i_, j_} /; Abs[i - j] == 1 → 1.},
  {2 nin + 1, 2 nin + 1}];
Ttot = ArrayFlatten[
  {{-D2 / (2 dt^2) + DiagonalMatrix[β μ t],
    DiagonalMatrix[β μ]},
  {DiagonalMatrix[β μ],
    -2. IdentityMatrix[2 nin + 1]}}];
Developer`PackedArrayQ[Ttot];

(* computation of the inverse,
this is done fast by Mathematica with
its internal codes,
in a different implementation one could
just invert a matrix with constant
diagonals, that can be done analitically *)

ITtot = Inverse[Ttot];
(*
Developer`PackedArrayQ[ITtot];
*)

(* Boundary conditions on the columns *)
Vin = ConstantArray[0.0, 2 (2 nin + 1)];
Vin[[1]] = 1.0;
Vfin = ConstantArray[0.0, 2 (2 nin + 1)];

```

```
Vfin[[2 nin + 1]] = 1.0;
```

```
(* The equations on the boundaries,
note that we have multiplied them by the
inverse of Ttot,
this is the essential preconditioning step *)
```

```
VCR1in = -Vin / (2 dt2);
```

```
VCR1fin = -Vfin / (2 dt2);
```

```
VR2Xin = -Vin / (4 dt2);
```

```
VR2Xfin = -Vfin / (4 dt2);
```

```
equaCR1in = -CR1in - ITtot.VCR1in - ITtot.pCR1in;
```

```
equaCR1fin = -CR1fin - ITtot.VCR1fin -
```

```
ITtot.pCR1fin;
```

```
equaR2Xin = -R2Xin - ITtot.VR2Xin - ITtot.pR2Xin;
```

```
equaR2Xfin = -R2Xfin - ITtot.VR2Xfin -
```

```
ITtot.pR2Xfin;
```

```
(* contributions of the initial conditions
to the internal equations *)
```

```
bterm =
```

```
Transpose[ConstantArray[ITtot[[1]],
```

```
2 (2 nin + 1)]] ×
```

```
ConstantArray[CR1in, 2 (2 nin + 1)] +
```

```
Transpose[ConstantArray[ITtot[[2 nin + 1]],
```

```
2 (2 nin + 1)]] ×
```

```
ConstantArray[CR1fin, 2 (2 nin + 1)];
```

```
bterm *= 1 / (2 dt2);
```

```
(* the internal equations multiplied by
Itot *)
```

```
equaint = -Ctotint + ITtot / dt + bterm -
  ITtot.prodint;
equaintdt = -Ctotintdt + bterm - ITtot.prodintdt;
```

```
(* the full equations are written combining
back the internal equations with the
column equations to have two matrices
with the structure of Ctot and Ctotdt *)
```

```
equa = ConstantArray[0.0,
  {2 (2 n + 1), 2 (2 n + 1)}];
equadt = ConstantArray[0.0,
  {2 (2 n + 1), 2 (2 n + 1)}];

equa[[1]] =
  Join[ArrayPad[Take[equaCR1in, 2 nin + 1],
    1, 0.0],
    ArrayPad[Take[equaCR1in, -(2 nin + 1)],
      1, 0.0]];
equa[[All, 1]] = equa[[1]];
equadt[[1]] = equa[[1]];
equadt[[All, 1]] = equa[[1]];
```

```
equa[[2 n + 1]] =
  Join[ArrayPad[Take[equaCR1fin, 2 nin + 1],
    1, 0.0],
    ArrayPad[Take[equaCR1fin, -(2 nin + 1)],
```



```

1, 0.0]]];
equa[[All, 2 n + 1]] = equa[[2 n + 1]];
equadt[[2 n + 1]] = equa[[2 n + 1]];
equadt[[All, 2 n + 1]] = equa[[2 n + 1]];

equa[[2 n + 2]] =
Join[ArrayPad[Take[equaR2Xin, 2 nin + 1],
1, 0.0],
ArrayPad[Take[equaR2Xin, -(2 nin + 1)],
1, 0.0]];
equa[[All, 2 n + 2]] = equa[[2 n + 2]];
equadt[[2 n + 2]] = equa[[2 n + 2]];
equadt[[All, 2 n + 2]] = equa[[2 n + 2]];

equa[[2 (2 n + 1)]] =
Join[ArrayPad[Take[equaR2Xfin, 2 nin + 1],
1, 0.0],
ArrayPad[Take[equaR2Xfin, -(2 nin + 1)],
1, 0.0]];
equa[[All, 2 (2 n + 1)]] = equa[[2 (2 n + 1)]];
equadt[[2 (2 n + 1)]] = equa[[2 (2 n + 1)]];
equadt[[All, 2 (2 n + 1)]] = equa[[2 (2 n + 1)]];

equa[[2 ;; 2 n, 2 ;; 2 n]] =
Take[equaint, 2 nin + 1, 2 nin + 1];
equadt[[2 ;; 2 n, 2 ;; 2 n]] =
Take[equaintdt, 2 nin + 1, 2 nin + 1];

equa[[2 ;; 2 n, 2 n + 3 ;; 4 n + 1]] =
Take[equaint, 2 nin + 1, -(2 nin + 1)];

```

```

equadt[[2 ;; 2 n, 2 n + 3 ;; 4 n + 1]] =
  Take[equaintdt, 2 nin + 1, -(2 nin + 1)];

equa[[2 n + 3 ;; 4 n + 1, 2 ;; 2 n]] =
  Take[equaint, -(2 nin + 1), 2 nin + 1];
equadt[[2 n + 3 ;; 4 n + 1, 2 ;; 2 n]] =
  Take[equaintdt, -(2 nin + 1), 2 nin + 1];

equa[[2 n + 3 ;; 4 n + 1, 2 n + 3 ;; 4 n + 1]] =
  Take[equaint, -(2 nin + 1), -(2 nin + 1)];
equadt[[2 n + 3 ;; 4 n + 1, 2 n + 3 ;; 4 n + 1]] =
  Take[equaintdt, -(2 nin + 1), -(2 nin + 1)];

```

```

(* The saddle-point equations imposing
   the condition on the diagonals of C and R,
   they allows to determine  $\mu$  and  $\mu_t$  *)
equa $\mu$  = 1. - Take[Diagonal[Ctotint], 2 nin + 1];
equa $\mu_t$  = 1. - Diagonal[Ctotint, 2 nin + 1] -
  Diagonal[Ctotint, -(2 nin + 1)];

```

```

(*
Developer`PackedArrayQ[equadt] ;
Developer`PackedArrayQ[equa] ;
*)

```

```

};

```

```
CalcoloJv[] := {
```

```
(* this function computes the Jacobian
of the equations applied to a difference
matrix dCtot and dCtotdt,
it is a straightforward explicit derivative
of CalcoloEquazioni[] *)
```

```
(* Computation of  $d\Delta$  *)
```

```
dCC = Take[dCtot, 2 n + 1, 2 n + 1];
dThR2 = Take[dCtot, 2 n + 1, -(2 n + 1)];
dThR1 = Take[dCtot, -(2 n + 1), 2 n + 1];
dT2hX = Take[dCtot, -(2 n + 1), -(2 n + 1)];
dCCdt = Take[dCtotdt, 2 n + 1, 2 n + 1];
dThR2dt = Take[dCtotdt, 2 n + 1, -(2 n + 1)];
dThR1dt = Take[dCtotdt, -(2 n + 1), 2 n + 1];
dT2hXdt = Take[dCtotdt, -(2 n + 1), -(2 n + 1)];
```

```

dΓCC = CC dCC;
dThΓR1 = CC dThR1 + dCC ThR1;
dThΓR2 = CC dThR2 + dCC ThR2;
dT2hΓX = dCC T2hX + CC dT2hX + dThR1 ThR2 +
  ThR1 dThR2;

dΓCtot =
  -3 β2 ArrayFlatten[
    {{dT2hΓX, dThΓR1}, {dThΓR2, dΓCC}}];
(*
Developer`PackedArrayQ[dΓCtot];
*)

dΓCCdt = CCdt dCCdt;
dThΓR1dt = CCdt dThR1dt + dCCdt ThR1dt;
dThΓR2dt = CCdt dThR2dt + dCCdt ThR2dt;
dT2hΓXdt = dCCdt T2hXdt + CCdt dT2hXdt +
  dThR1dt ThR2dt + ThR1dt dThR2dt;

dΓCtotdt =
  -3 β2 ArrayFlatten[
    {{dT2hΓXdt, dThΓR1dt},
     {dThΓR2dt, dΓCCdt }}];

(*
Developer`PackedArrayQ[dΓCtotdt];
*)
(*****

(*****

(* the differential of the interaction
term *)

```

```

hprod = rCtotdt.dCtotdt + d rCtotdt.Ctotdt;
dprod = d rCtot.Ctot - hprod + rCtot.dCtot;
dproddt = d rCtot.Ctotdt + d rCtotdt.Ctot -
    2 hprod + rCtot.dCtotdt + rCtotdt.dCtot;
dprod *= dt;
dproddt *= dt;

```

```

dPP =
  Flatten[Take[d rCtot, 2 (2 n + 1),
    {(2 n + 1) + 1}]] ×
    ConstantArray[Take[Ctot, 1][[1]], 2 (2 n + 1)]
+
  Flatten[Take[rCtot, 2 (2 n + 1),
    {(2 n + 1) + 1}]] ×
    ConstantArray[Take[dCtot, 1][[1]],
      2 (2 n + 1)];

```

```

dPP +=
  Flatten[Take[d rCtot, 2 (2 n + 1), {2 (2 n + 1)}]] ×
    ConstantArray[Take[Ctot, {2 n + 1}][[1]],
      2 (2 n + 1)] +
  Flatten[Take[rCtot, 2 (2 n + 1), {2 (2 n + 1)}]] ×
    ConstantArray[Take[dCtot, {2 n + 1}][[1]],
      2 (2 n + 1)];

```

```

dprod += dPP;
dproddt += dPP;

```

```

(*
Developer`PackedArrayQ[dprod];
Developer`PackedArrayQ[dproddt];

```

```

*)

(*****)

(* internal part of the interaction term *)
dprodint = ArrayFlatten[
  {{dprod[[2 ;; 2 n, 2 ;; 2 n]],
    dprod[[2 ;; 2 n, 2 n + 3 ;; 4 n + 1]]},
  {dprod[[2 n + 3 ;; 4 n + 1, 2 ;; 2 n]],
    dprod[[2 n + 3 ;; 4 n + 1, 2 n + 3 ;; 4 n + 1]]}}];
dprodintdt = ArrayFlatten[
  {{dproddt[[2 ;; 2 n, 2 ;; 2 n]],
    dproddt[[2 ;; 2 n, 2 n + 3 ;; 4 n + 1]]},
  {dproddt[[2 n + 3 ;; 4 n + 1, 2 ;; 2 n]],
    dproddt[[2 n + 3 ;; 4 n + 1,
      2 n + 3 ;; 4 n + 1]]}}];
(*****)
(* boundaries of the interaction terms *)
dpCR1in = Join[dprod[[2 ;; 2 n, 1]],
  dprod[[2 n + 3 ;; 4 n + 1, 1]]];
dpCR1fin = Join[dprod[[2 ;; 2 n, 2 n + 1]],
  dprod[[2 n + 3 ;; 4 n + 1, 2 n + 1]]];
dpR2Xin = Join[dprod[[2 ;; 2 n, 2 n + 2]],
  dprod[[2 n + 3 ;; 4 n + 1, 2 n + 2]]];
dpR2Xfin = Join[dprod[[2 ;; 2 n, 4 n + 2]],
  dprod[[2 n + 3 ;; 4 n + 1, 4 n + 2]]];

(* internal part of the differentials *)
dCtotint = ArrayFlatten[
  {{dCtot[[2 ;; 2 n, 2 ;; 2 n]],
    dCtot[[2 ;; 2 n, 2 n + 3 ;; 4 n + 1]]},
  {dCtot[[2 n + 3 ;; 4 n + 1, 2 ;; 2 n]],
    dCtot[[2 n + 3 ;; 4 n + 1, 2 n + 3 ;; 4 n + 1]]}}];

```

```

dCtotintdt = ArrayFlatten[
  {{dCtotdt[[2 ;; 2 n, 2 ;; 2 n]],
    dCtotdt[[2 ;; 2 n, 2 n + 3 ;; 4 n + 1]]},
  {dCtotdt[[2 n + 3 ;; 4 n + 1, 2 ;; 2 n]],
    dCtotdt[[2 n + 3 ;; 4 n + 1,
      2 n + 3 ;; 4 n + 1]]}}];
(*****
(* boundary parts of the differentials *)
dCR1in = Join[dCtot[[2 ;; 2 n, 1]],
  dCtot[[2 n + 3 ;; 4 n + 1, 1]]];
dCR1fin = Join[dCtot[[2 ;; 2 n, 2 n + 1]],
  dCtot[[2 n + 3 ;; 4 n + 1, 2 n + 1]]];
dR2Xin = Join[dCtot[[2 ;; 2 n, 2 n + 2]],
  dCtot[[2 n + 3 ;; 4 n + 1, 2 n + 2]]];
dR2Xfin = Join[dCtot[[2 ;; 2 n, 4 n + 2]],
  dCtot[[2 n + 3 ;; 4 n + 1, 4 n + 2]]];

(*****

(* Differential of the term involving
the second derivatives *)

dTtot = ArrayFlatten[
  {{DiagonalMatrix[dβμt], DiagonalMatrix[dβμ]},
  {DiagonalMatrix[dβμ],
    0.0 IdentityMatrix[2 nin + 1]}}];
(*Developer`PackedArrayQ[Ttot];*)

dITtot = -ITtot.dTtot.ITtot;
(*Developer`PackedArrayQ[ITtot];*)

```

```
(* differential of the equations on the
boundaries *)
```

```
(*****)
```

```
dequaCR1in = -dCR1in - dITtot.VCR1in -
  dITtot.pCR1in - ITtot.dpCR1in;
dequaCR1fin = -dCR1fin - dITtot.VCR1fin -
  dITtot.pCR1fin - ITtot.dpCR1fin;
dequaR2Xin = -dR2Xin - dITtot.VR2Xin -
  dITtot.pR2Xin - ITtot.dpR2Xin;
dequaR2Xfin = -dR2Xfin - dITtot.VR2Xfin -
  dITtot.pR2Xfin - ITtot.dpR2Xfin;
```

```
(*****)
```

```
(* differential of the boundary terms
on the internal equations *)
```

```
dbterm =
  Transpose[ConstantArray[dITtot[[1]],
    2 (2 nin + 1)]] ×
  ConstantArray[CR1in, 2 (2 nin + 1)] +
  Transpose[ConstantArray[ITtot[[1]],
    2 (2 nin + 1)]] ×
  ConstantArray[dCR1in, 2 (2 nin + 1)] +
  Transpose[ConstantArray[dITtot[[2 nin + 1]],
    2 (2 nin + 1)]] ×
  ConstantArray[CR1fin, 2 (2 nin + 1)] +
  Transpose[ConstantArray[ITtot[[2 nin + 1]],
    2 (2 nin + 1)]] ×
  ConstantArray[dCR1fin, 2 (2 nin + 1)];
dbterm *= 1 / (2 dt2);
```



```
(* differential of the internal equations *)
```

```
dequaint = -dCtotint + dITtot / dt + dbterm -  
            dITtot.prodint - ITtot.dprodint;  
dequaintdt = -dCtotintdt + dbterm -  
              dITtot.prodintdt - ITtot.dprodintdt;
```

```
(* differential of the full equations *)
```

```
dequa = ConstantArray[0.0,  
    {2 (2 n + 1), 2 (2 n + 1)}];  
dequadt = ConstantArray[0.0,  
    {2 (2 n + 1), 2 (2 n + 1)}];  
  
dequa[[1]] =  
    Join[ArrayPad[Take[dequaCR1in, 2 nin + 1],  
        1, 0.0],  
        ArrayPad[Take[dequaCR1in, -(2 nin + 1)],  
            1, 0.0]];  
dequa[[All, 1]] = dequa[[1]];  
dequadt[[1]] = dequa[[1]];  
dequadt[[All, 1]] = dequa[[1]];
```

```
dequa[[2 n + 1]] =  
    Join[ArrayPad[Take[dequaCR1fin, 2 nin + 1],  
        1, 0.0],  
        ArrayPad[Take[dequaCR1fin, -(2 nin + 1)],
```

```

1, 0.0]]];
dequa[[All, 2 n + 1]] = dequa[[2 n + 1]];
dequadt[[2 n + 1]] = dequa[[2 n + 1]];
dequadt[[All, 2 n + 1]] = dequa[[2 n + 1]];

dequa[[2 n + 2]] =
Join[ArrayPad[Take[dequaR2Xin, 2 nin + 1],
1, 0.0],
ArrayPad[Take[dequaR2Xin, -(2 nin + 1)],
1, 0.0]];
dequa[[All, 2 n + 2]] = dequa[[2 n + 2]];
dequadt[[2 n + 2]] = dequa[[2 n + 2]];
dequadt[[All, 2 n + 2]] = dequa[[2 n + 2]];

dequa[[2 (2 n + 1)]] =
Join[ArrayPad[Take[dequaR2Xfin, 2 nin + 1],
1, 0.0],
ArrayPad[Take[dequaR2Xfin, -(2 nin + 1)],
1, 0.0]];
dequa[[All, 2 (2 n + 1)]] = dequa[[2 (2 n + 1)]];
dequadt[[2 (2 n + 1)]] = dequa[[2 (2 n + 1)]];
dequadt[[All, 2 (2 n + 1)]] = dequa[[2 (2 n + 1)]];

dequa[[2 ;; 2 n, 2 ;; 2 n]] =
Take[dequaint, 2 nin + 1, 2 nin + 1];
dequadt[[2 ;; 2 n, 2 ;; 2 n]] =
Take[dequaintdt, 2 nin + 1, 2 nin + 1];

dequa[[2 ;; 2 n, 2 n + 3 ;; 4 n + 1]] =
Take[dequaint, 2 nin + 1, -(2 nin + 1)];

```

```

dequadt[[2 ;; 2 n, 2 n + 3 ;; 4 n + 1]] =
  Take[dequaintdt, 2 nin + 1, -(2 nin + 1)];

dequa[[2 n + 3 ;; 4 n + 1, 2 ;; 2 n]] =
  Take[dequaint, -(2 nin + 1), 2 nin + 1];
dequadt[[2 n + 3 ;; 4 n + 1, 2 ;; 2 n]] =
  Take[dequaintdt, -(2 nin + 1), 2 nin + 1];

dequa[[2 n + 3 ;; 4 n + 1, 2 n + 3 ;; 4 n + 1]] =
  Take[dequaint, -(2 nin + 1), -(2 nin + 1)];
dequadt[[2 n + 3 ;; 4 n + 1, 2 n + 3 ;; 4 n + 1]] =
  Take[dequaintdt, -(2 nin + 1), -(2 nin + 1)];

(* differential of the equations for  $\mu$ 
   and  $\mu_t$  *)
dequa $\mu$  = -Take[Diagonal[dCtotint], 2 nin + 1];
dequa $\mu_t$  = -Diagonal[dCtotint, 2 nin + 1] -
  Diagonal[dCtotint, -(2 nin + 1)];

(*

Developer`PackedArrayQ[dequadt] ;
Developer`PackedArrayQ[dequa] ;

*)

};

```

```
(** Definitions of the norms **)
```

```
Prod2[a1_, a2_] :=
  Total[(a1[[1]] × a2[[1]] + a1[[2]] × a2[[2]]), 2] -
  3. (a1[[1]][[1]].a2[[1]][[1]] +
      a1[[1]][[2 n + 1]].a2[[1]][[2 n + 1]] +
      a1[[1]][[2 n + 2]].a2[[1]][[2 n + 2]] +
      a1[[1]][[4 n + 2]].a2[[1]][[4 n + 2]]) +
  Total[a1[[3]] × a2[[3]]] +
  Total[a1[[4]] × a2[[4]]];
```

```
Norm2[a1_] :=
  (Norm[a1[[1]], "Frobenius"]2 +
   Norm[a1[[2]], "Frobenius"]2 -
   3 (Norm[a1[[1]][[1]]]2 +
      Norm[a1[[1]][[2 n + 1]]]2 +
      Norm[a1[[1]][[2 n + 2]]]2 +
      Norm[a1[[1]][[4 n + 2]]]2) +
  Norm[a1[[3]]]2 + Norm[a1[[4]]]2).5;
```

```
(* the GMRES algorithm *)
```

```
GMRES[sres_, nKmax_] := {
```

```

(***** GMRES *****)
Clear[q]; (* q is the Arnoldi base *)
q[1] = -{equa, equadt, equa $\mu$ , equa $\mu$ t};
h[1, 0] = Norm2[q[1]];
q[1] /= h[1, 0];
{dCtot, dCtotdt, d $\beta\mu$ , d $\beta\mu$ t} = q[1];
res0 = h[1, 0];
res = res0;
(* nKmax max size of the Krylov subspace *)

For[k = 2, res > sres res0 && k ≤ nKmax + 1,

  CalcoloJv[]; (* compute the new element
    of the Krylov subspace *)

  (* Arnoldi *)

  q[k] = {dequa, dequadt, dequa $\mu$ , dequa $\mu$ t};

  Do[
    h[j, k - 1] = Prod2[q[j], q[k]];
    q[k] = q[k] - h[j, k - 1] × q[j];
    , {j, 1, k - 1}];

  h[k, k - 1] = Norm2[q[k]];
  q[k] /= h[k, k - 1];

  Do[h[j, k - 1] = 0.0, {j, k + 1, nKmax + 1}];

  (*****)

  {dCtot, dCtotdt, d $\beta\mu$ , d $\beta\mu$ t} = q[k];

```

```

(**least squares to minimize the residue *)

tHn = Array[h, {k, k - 1}];
βe = Table[0.0, {i, 1, k}];
βe[[1]] = h[1, 0];
yn = LeastSquares[tHn, βe];
(*Mathematica does this internally,
a different implementation would require
to specify the procedure *)
res = Norm[tHn.yn - βe];
(* PrintTemporary[res]; *)

k++;

];
k--;
nK = k
(* the effective nK,
in case one fixes a target on the residue
sres *)
};

```

```

(* symmetrizing functions *)

SymR2[X_] := (
  X + Reverse[X, {1, 2}]
  (* symmetrized with respect to the
     exchange of the initial and final points
     but it is DOUBLED hence the 2*)
);

(* function that symmetrize its argument,
example FullSym[Ctot], FullSym[Ctotdt],
FullSym[equadt]... *)
SetAttributes[FullSym, HoldFirst];
FullSym[X_] := (
  X = ArrayFlatten[
    {{SymR2[Take[X, 2 n + 1, 2 n + 1]],
      SymR2[Take[X, 2 n + 1, -(2 n + 1)]]},
     {SymR2[Take[X, -(2 n + 1), 2 n + 1]],
      SymR2[Take[X, -(2 n + 1), -(2 n + 1)]]}}];
  X += Transpose[X];
  X *= .25;
);

(* function that symmetrize its argument,
example SymV[βμ], SymV[equaμ]... *)
SetAttributes[SymV, HoldFirst];
SymV[X_] := (X += Reverse[X]; X *= .5);

(** Compression and decompression functions

```

```

    for the C and the X,
    the original matrices are store into smaller
    objects exploiting the symmetries,
    see manuscript **)

```

```

Comp[X_] :=
  LowerTriangularize[Take[X, n + 1, n + 1]] +
  PadLeft[UpperTriangularize[
    Reverse[Take[X, n, -n], 2]], {-(n + 1), n + 1},
    0.0];

```

```

(* inverse *)

```

```

IComp[X_] := (
  OR1 = LowerTriangularize[X];
  OR1 =
    OR1 + Transpose[LowerTriangularize[OR1, -1]];
  OR2 = Drop[UpperTriangularize[X, 1], -1, 1];
  OR2 =
    OR2 + Transpose[UpperTriangularize[OR2, 1]];
  OR2 = Reverse[OR2, 2];
  AppendTo[OR2, Reverse[Drop[Last[OR1], -1]]];
  ArrayFlatten[
    {{OR1, OR2}, {Transpose[OR2],
      Drop[Reverse[OR1, {1, 2}], 1, 1]}}]
);

```

```

(* compression and decompress for the R *)

```

```

CompR[X_] := {Take[X, n + 1, n + 1], Take[X, n, -n]};

```

```

ICompR[X_] := (

```



```

OR1 = X[[1]];
OR2 = X[[2]];
OR2 = AppendTo[OR2,
  Reverse[Drop[Last[OR1], -1]]];
OR2b = Reverse[X[[2]], {1, 2}];
OR2b = Transpose[OR2b];
OR2b = AppendTo[OR2b,
  Reverse[Drop[OR1[[All, n + 1]], -1]]];
ArrayFlatten[
  {{OR1, OR2}, {Transpose[OR2b],
    Drop[Reverse[OR1, {1, 2}], 1, 1]}}]]

(*  $\mu \in \mu^t$  *)

Compvec[X_] := Take[X, nin + 1];
ICompvec[X_] := Join[X, Reverse[Drop[X, -1]]];

(** Complete compression function to be
    applied to an object of the form
    {equa, equadt, equa $\mu$ , equa $\mu^t$ } **)

FullComp[X_] := (
  a1 = Comp[Take[X[[1]], 2 n + 1, 2 n + 1]];
  a2 = CompR[Take[X[[1]], (2 n + 1), -(2 n + 1)]];
  a3 = Comp[Take[X[[1]], -(2 n + 1), -(2 n + 1)]];

  a1dt = Drop[Comp[Take[X[[2]], 2 n + 1, 2 n + 1]],
    1, 1];
  ab = CompR[Take[X[[2]], (2 n + 1), -(2 n + 1)]];
  a2dt = {Drop[ab[[1]], 1, 1],
    Drop[ab[[2]], 1, -1]};

```

```

a3dt = Comp[Take[X[[2]], -(2 n + 1), -(2 n + 1)]];
{{a1, a2, a3},
 {a1dt, a2dt, a3dt}, Compvec[X[[3]]],
 Compvec[X[[4]]]}
);

```

(\* Inverse of the full compression,  
it gives back an object four times larger \*)

```

IFullComp[X_] := (
  a1 = IComp[X[[1, 1]]];
  a2 = ICompR[X[[1, 2]]];
  a3 = IComp[X[[1, 3]]];

  a1dt = PadLeft[X[[2, 1]], {n + 1, n + 1}, 0.0];
  a1dt[[1]] = X[[1, 1]][[1]];
  a1dt[[All, 1]] = X[[1, 1]][[All, 1]];
  a1dt = IComp[a1dt];

  a2dt = {PadLeft[X[[2, 2, 1]], {n + 1, n + 1}, 0.0],
    PadLeft[X[[2, 2, 2]], {n, -n}, 0.0]};
  a2dt[[1, 1]] = X[[1, 2, 1]][[1]];
  a2dt[[1, All, 1]] = X[[1, 2, 1]][[All, 1]];
  a2dt[[2, 1]] = X[[1, 2, 2]][[1]];
  a2dt[[2, All, n]] = X[[1, 2, 2]][[All, n]];
  a2dt = ICompR[a2dt];

  a3dt = PadLeft[X[[2, 3]], {n + 1, n + 1}, 0.0];
  a3dt[[1]] = X[[1, 3]][[1]];
  a3dt[[All, 1]] = X[[1, 3]][[All, 1]];
  a3dt = IComp[a3dt];
{

```

```

    ArrayFlatten[{{a1, a2}, {Transpose[a2], a3}}]
  ,
  ArrayFlatten[
    {{a1dt, a2dt}, {Transpose[a2dt], a3dt}}]
  ,
  ICompvec[X[[3]]], ICompvec[X[[4]]]
);

```

(\* GMRES using compressed matrices \*)

```

GMREScomp[sres_, nKmax_] := {
  (***** GMRES *****)
  Clear[q];
  q[1] =
    FullComp[-{equa, equadt, equa $\mu$ , equa $\mu$ t}];
  h[1, 0] = Total[q[1]2, Infinity].5;
  (* no element is repeated in q thus the
    norm is the standard norm *)
  q[1] /= h[1, 0];
  {dCtot, dCtotdt, d $\beta\mu$ , d $\beta\mu$ t} =
    IFullComp[q[1]];
  res0 = h[1, 0];
  res = res0;
  (* nKmax max size of the Krylov subspace *)

  For[k = 2, res > sres res0 && k ≤ nKmax + 1,

    CalcoloJv[]; (* compute the new element
      of the Krylov subspace *)
    (* symmetrizing the output *)
    FullSym[dequa];

```

```

FullSym[dequadt];
SymV[dequa $\mu$ ];
SymV[dequa $\mu$ t];

(* Arnoldi *)

q[k] = FullComp[{dequa, dequadt, dequa $\mu$ ,
  dequa $\mu$ t}]; (* compressing the output *)

Do[
  h[j, k - 1] = Total[q[j]  $\times$  q[k], Infinity];
  q[k] = q[k] - h[j, k - 1]  $\times$  q[j];
  , {j, 1, k - 1}];

h[k, k - 1] = Total[q[k]2, Infinity].5;
q[k] /= h[k, k - 1];

Do[h[j, k - 1] = 0.0, {j, k + 1, nKmax + 1}];

(*****)

{dCtot, dCtotdt, d $\beta\mu$ , d $\beta\mu$ t} = IFullComp[q[k]];

(**least squares to minimize the residue *)

tHn = Array[h, {k, k - 1}];
 $\beta$ e = Table[0.0, {i, 1, k}];
 $\beta$ e[[1]] = h[1, 0];
yn = LeastSquares[tHn,  $\beta$ e];
res = Norm[tHn.yn -  $\beta$ e];
(* PrintTemporary[res]; *)

```

```

    k++;

];
k--;
nK = k
(* effective nK *)
};

```

```
CalcoloEE[] := (
```

```

    (* this compute the derivative of the
       log rate with respect to  $\beta$  *)

```

```

CC = Take[Ctot, 2 n + 1, 2 n + 1];
ThR2 = Take[Ctot, 2 n + 1, -(2 n + 1)];
ThR1 = Take[Ctot, -(2 n + 1), 2 n + 1];
T2hX = Take[Ctot, -(2 n + 1), -(2 n + 1)];
CCdt = Take[Ctotdt, 2 n + 1, 2 n + 1];
ThR2dt = Take[Ctotdt, 2 n + 1, -(2 n + 1)];
ThR1dt = Take[Ctotdt, -(2 n + 1), 2 n + 1];
T2hXdt = Take[Ctotdt, -(2 n + 1), -(2 n + 1)];

```

```

ER1 = 3 / 2  $\beta$  CC2 ThR1;
EX = 3 / 2  $\beta$  CC2 T2hX + 3  $\beta$  CC ThR1 ThR2;
EXdt = 3 / 2  $\beta$  CCdt2 T2hXdt +
      3  $\beta$  CCdt ThR1dt ThR2dt;

```

```

4 (Total[ER1[[;;, 1]]] - (3 / 2  $\beta$  1.  $\times$  .5) .5) dt +

```

```
(Total[EX, Infinity] - Total[EXdt, Infinity])
dt2
```

```
(* (3/2 β 1. .5).5 is to make the integral
valid a second order in dt by taking
care of the border effect. It is not
needed for the second part because the
border cancel due to the factor n-1 *)
```

```
(* this quantity should be equal to β/2
in the ergodic regime *)
```

```
);
```
